# Supplementary material for: Deep Smartphone Sensors-WiFi Fusion for Indoor Positioning and Tracking
Source: arXiv:2011.10799 source file (2020-11-21)
Supplement: Supplementary file 1 [file appendix.tex]

\section{Introduction}
